# Supplementary material for: RaD-VIO: Rangefinder-aided Downward Visual-Inertial Odometry
Source: arXiv:1810.08704 source file (2019-05-14)
Supplement: Supplementary file 1 [file supplementary.tex]

\section{Supplementary Material}

Representative video: {\color{magenta}https://youtu.be/gmFKWQCd1us}
